# Supplementary material for: HRT1: One-Shot Human-to-Robot Trajectory Transfer for Mobile Manipulation
Source: arXiv:2510.21026 source file (2025-10-23)
Supplement: Supplementary file 1 [file 7-appendix.tex]

\appendix

\begin{figure*}
    \centering
    \includegraphics[width=\linewidth,trim={0 7cm 0cm 0cm},clip]{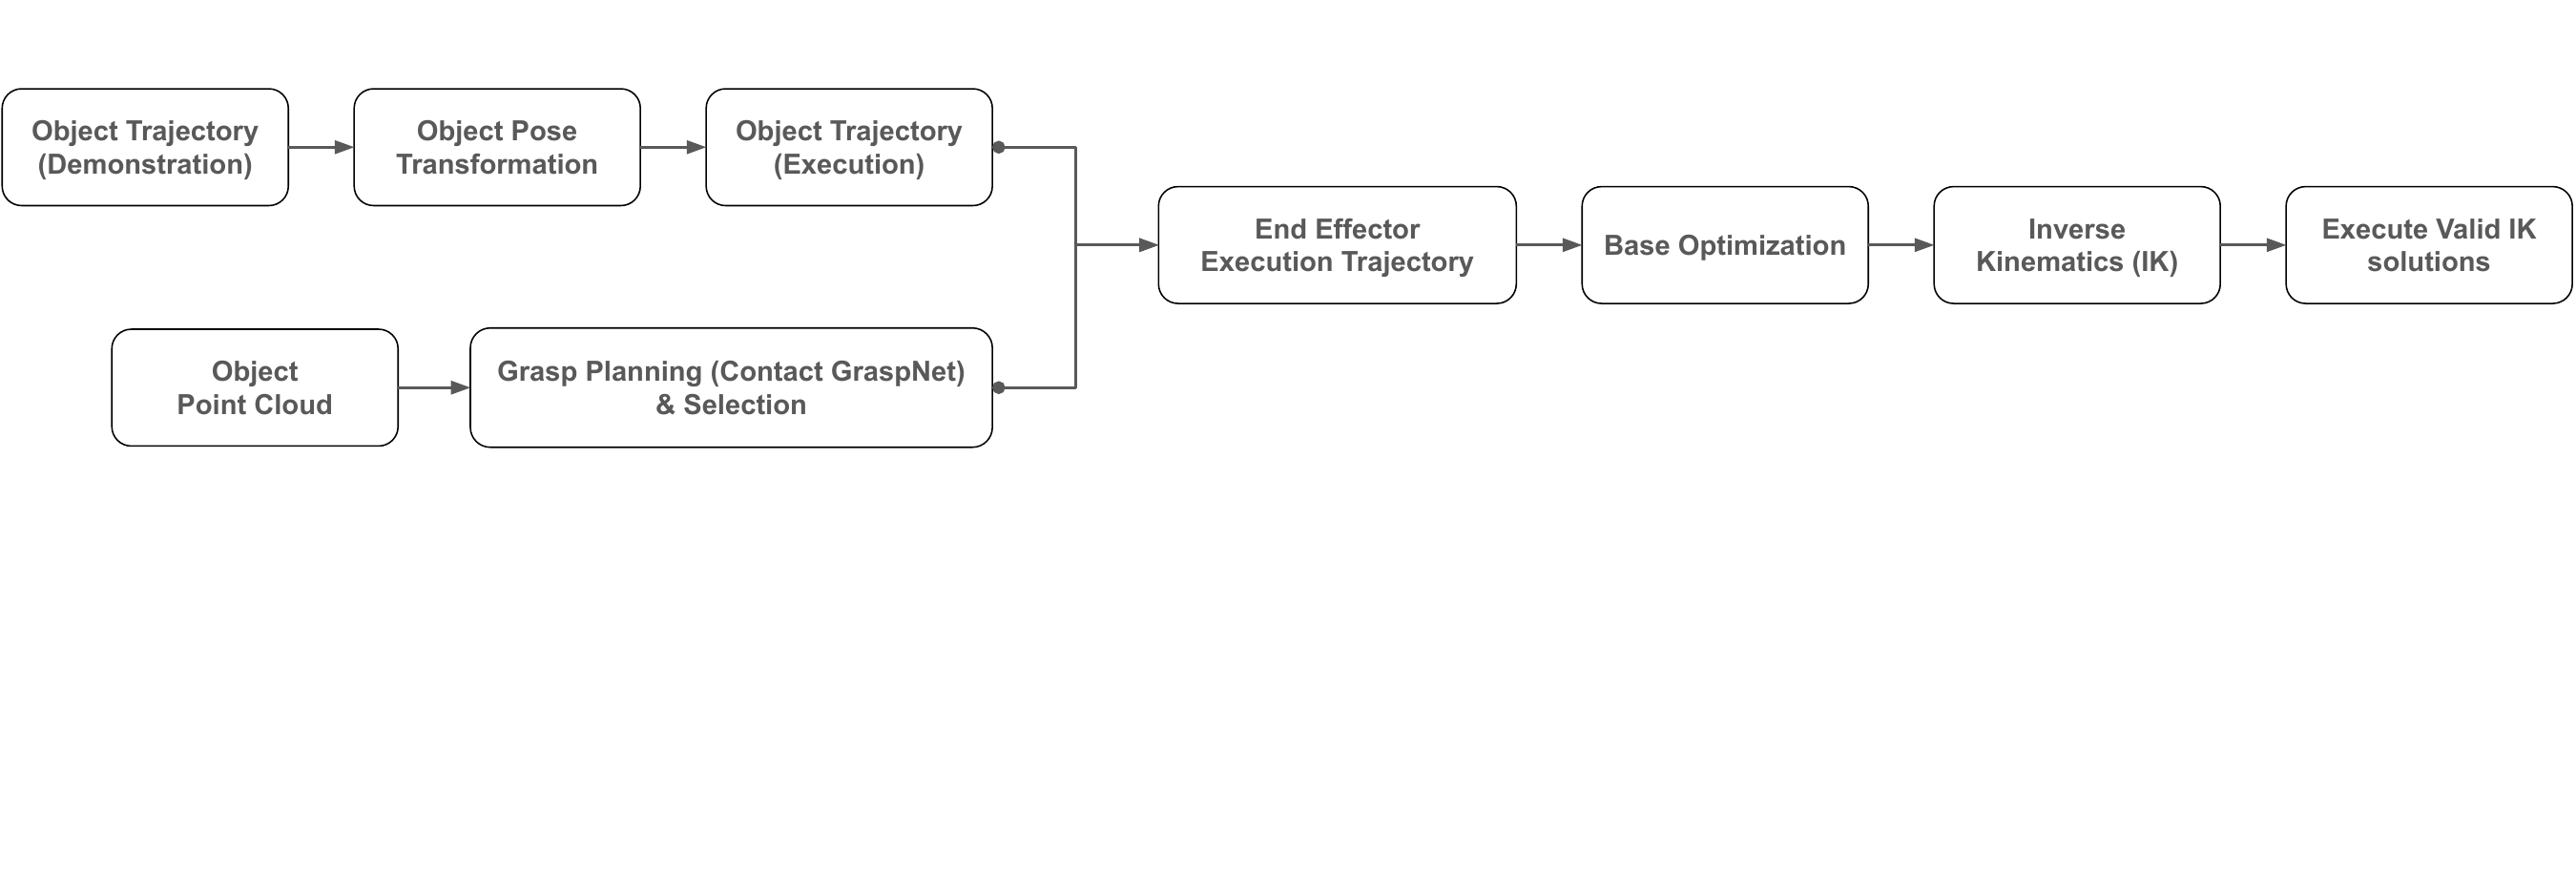}
    \caption{Baseline implementation Pipeline based on DITTO~\cite{heppert2024ditto}}
    \label{fig:baseline-pipeline}    
\end{figure*}

\begin{figure*}[ht]
    \centering
    \includegraphics[width=\linewidth]{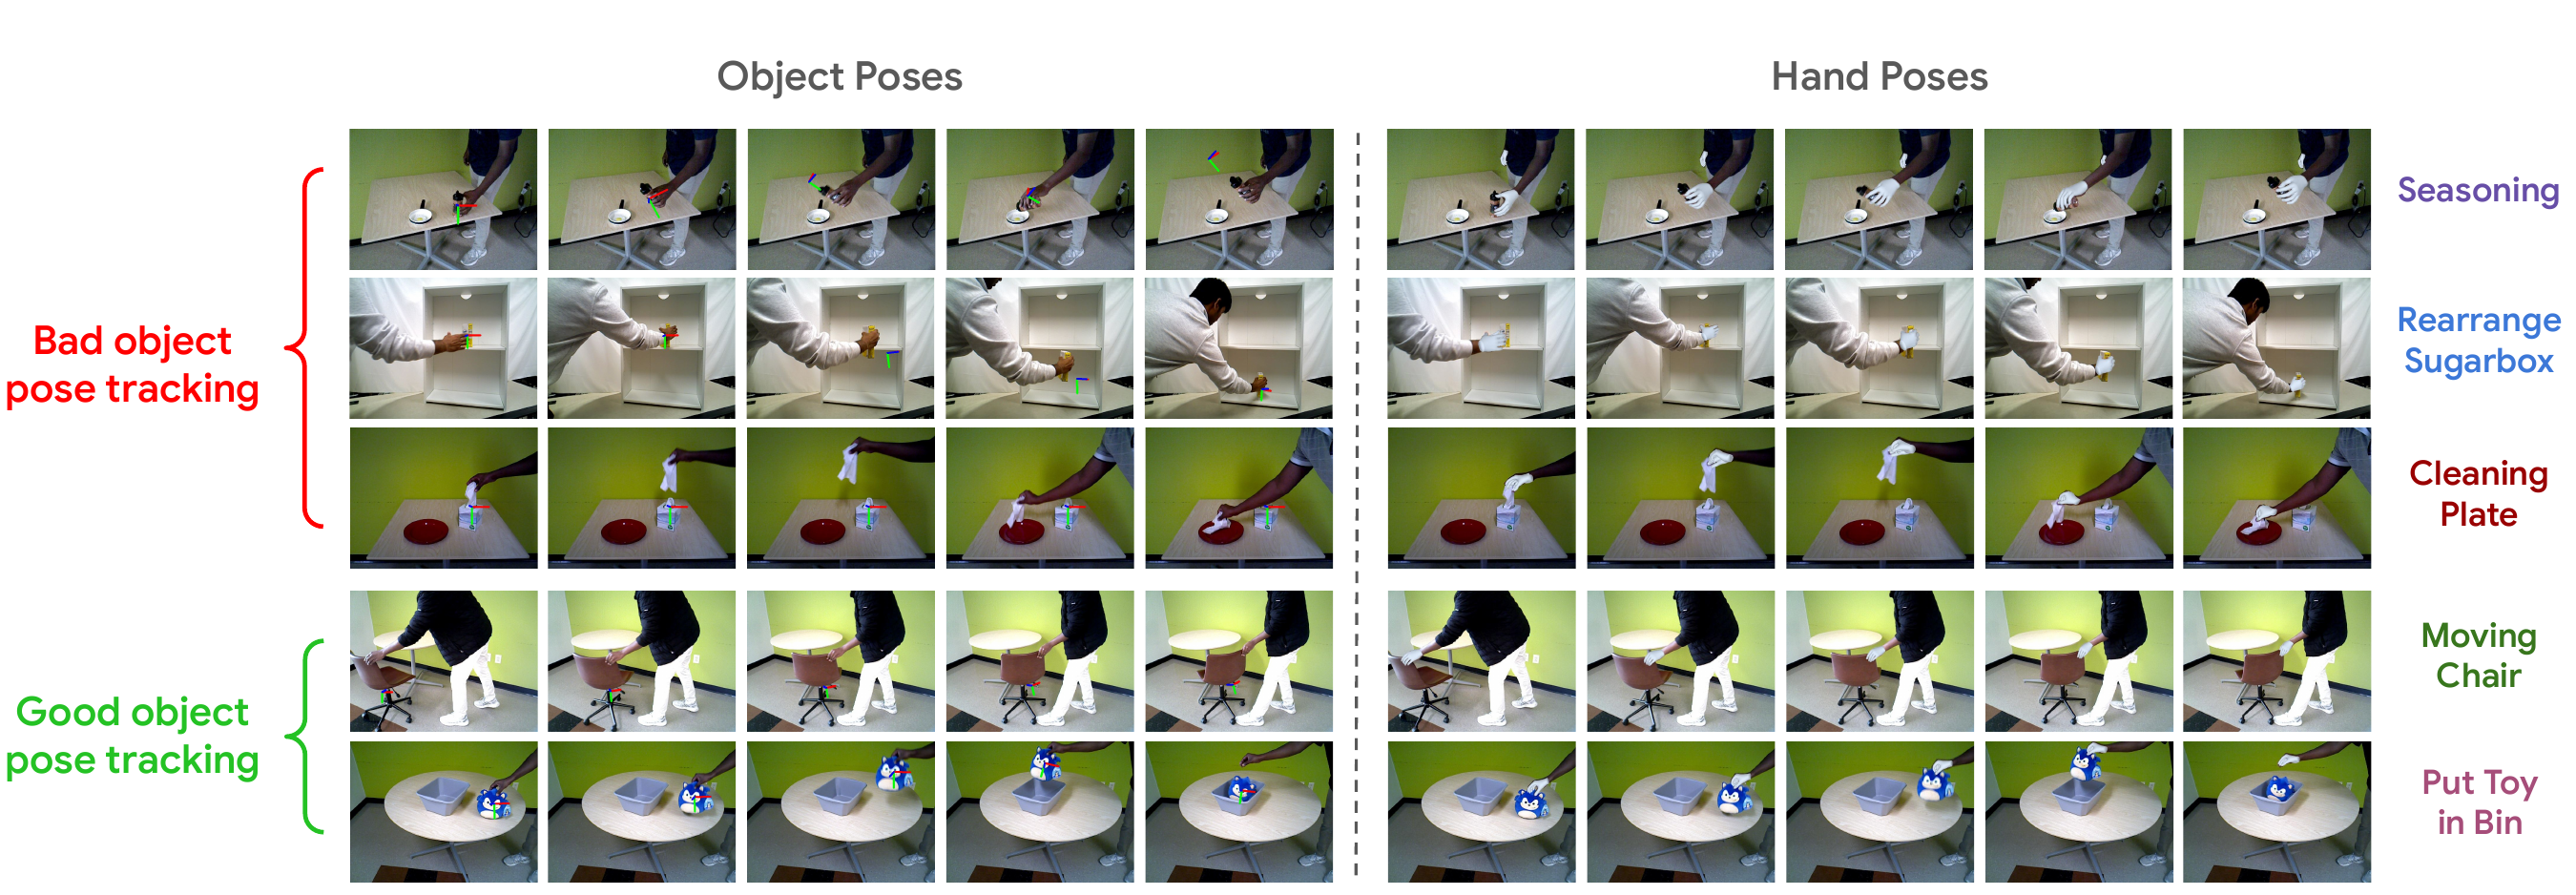}
    \caption{Comparison of Object poses and Human hand poses predicted in the demonstration frames.}
    \label{fig:hand-vs-obj-demo}
\end{figure*}

\begin{figure*}[ht]
    \centering
    \includegraphics[width=\linewidth,trim={5cm 0cm 0cm 0cm},clip]{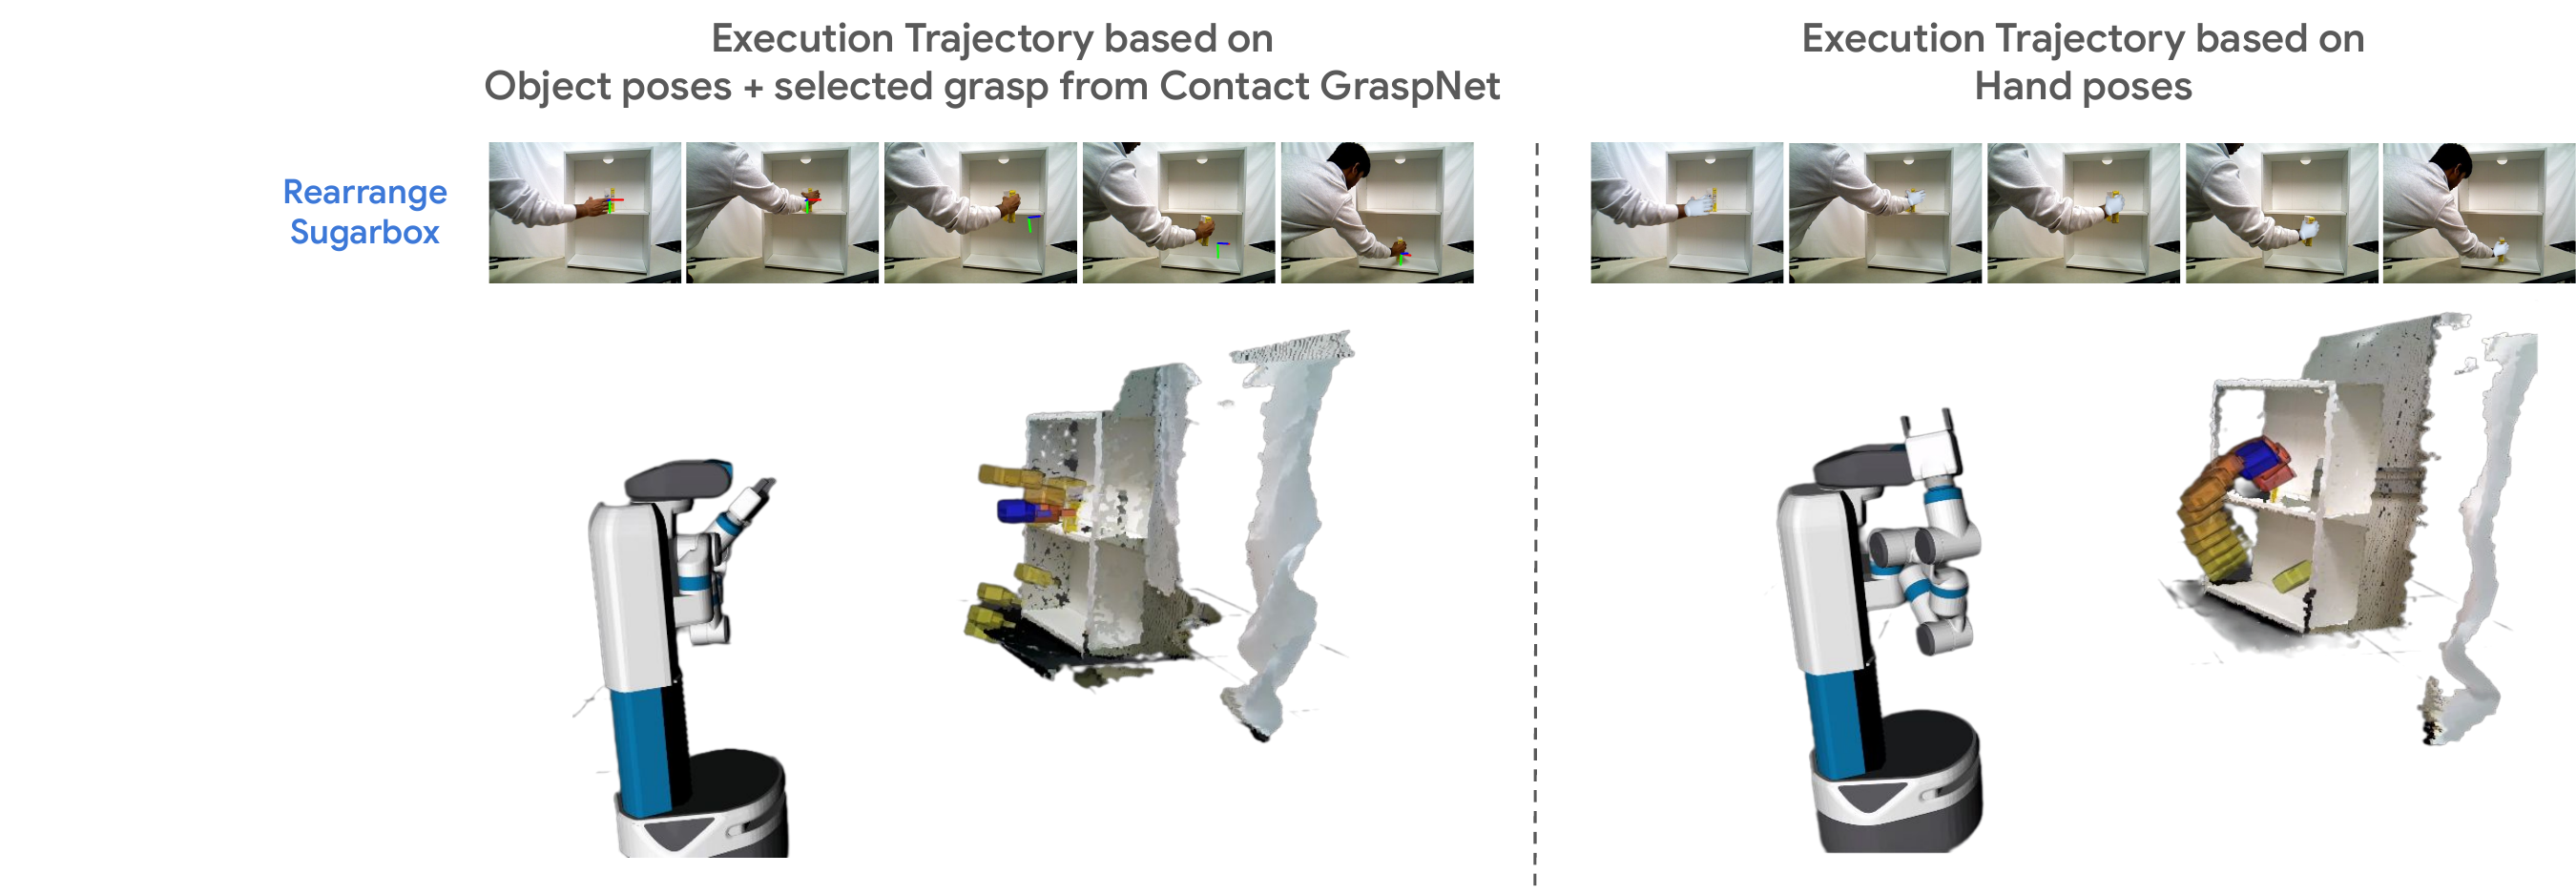}
    \caption{Visualization of execution trajectories of task \textit{rearrange sugar box}. (left) Erratic Baseline execution trajectory based on object poses and nearest grasp selected using Contact-GraspNet. (right) Stable and smooth execution trajectory of our method HRT1, based on hand pose transfer.}
    \label{fig:exec-hand-vs-obj-traj}
\end{figure*}

\begin{figure*}[ht]
    \centering
    \includegraphics[width=\linewidth,trim={3cm 0cm 0cm 0cm},clip]{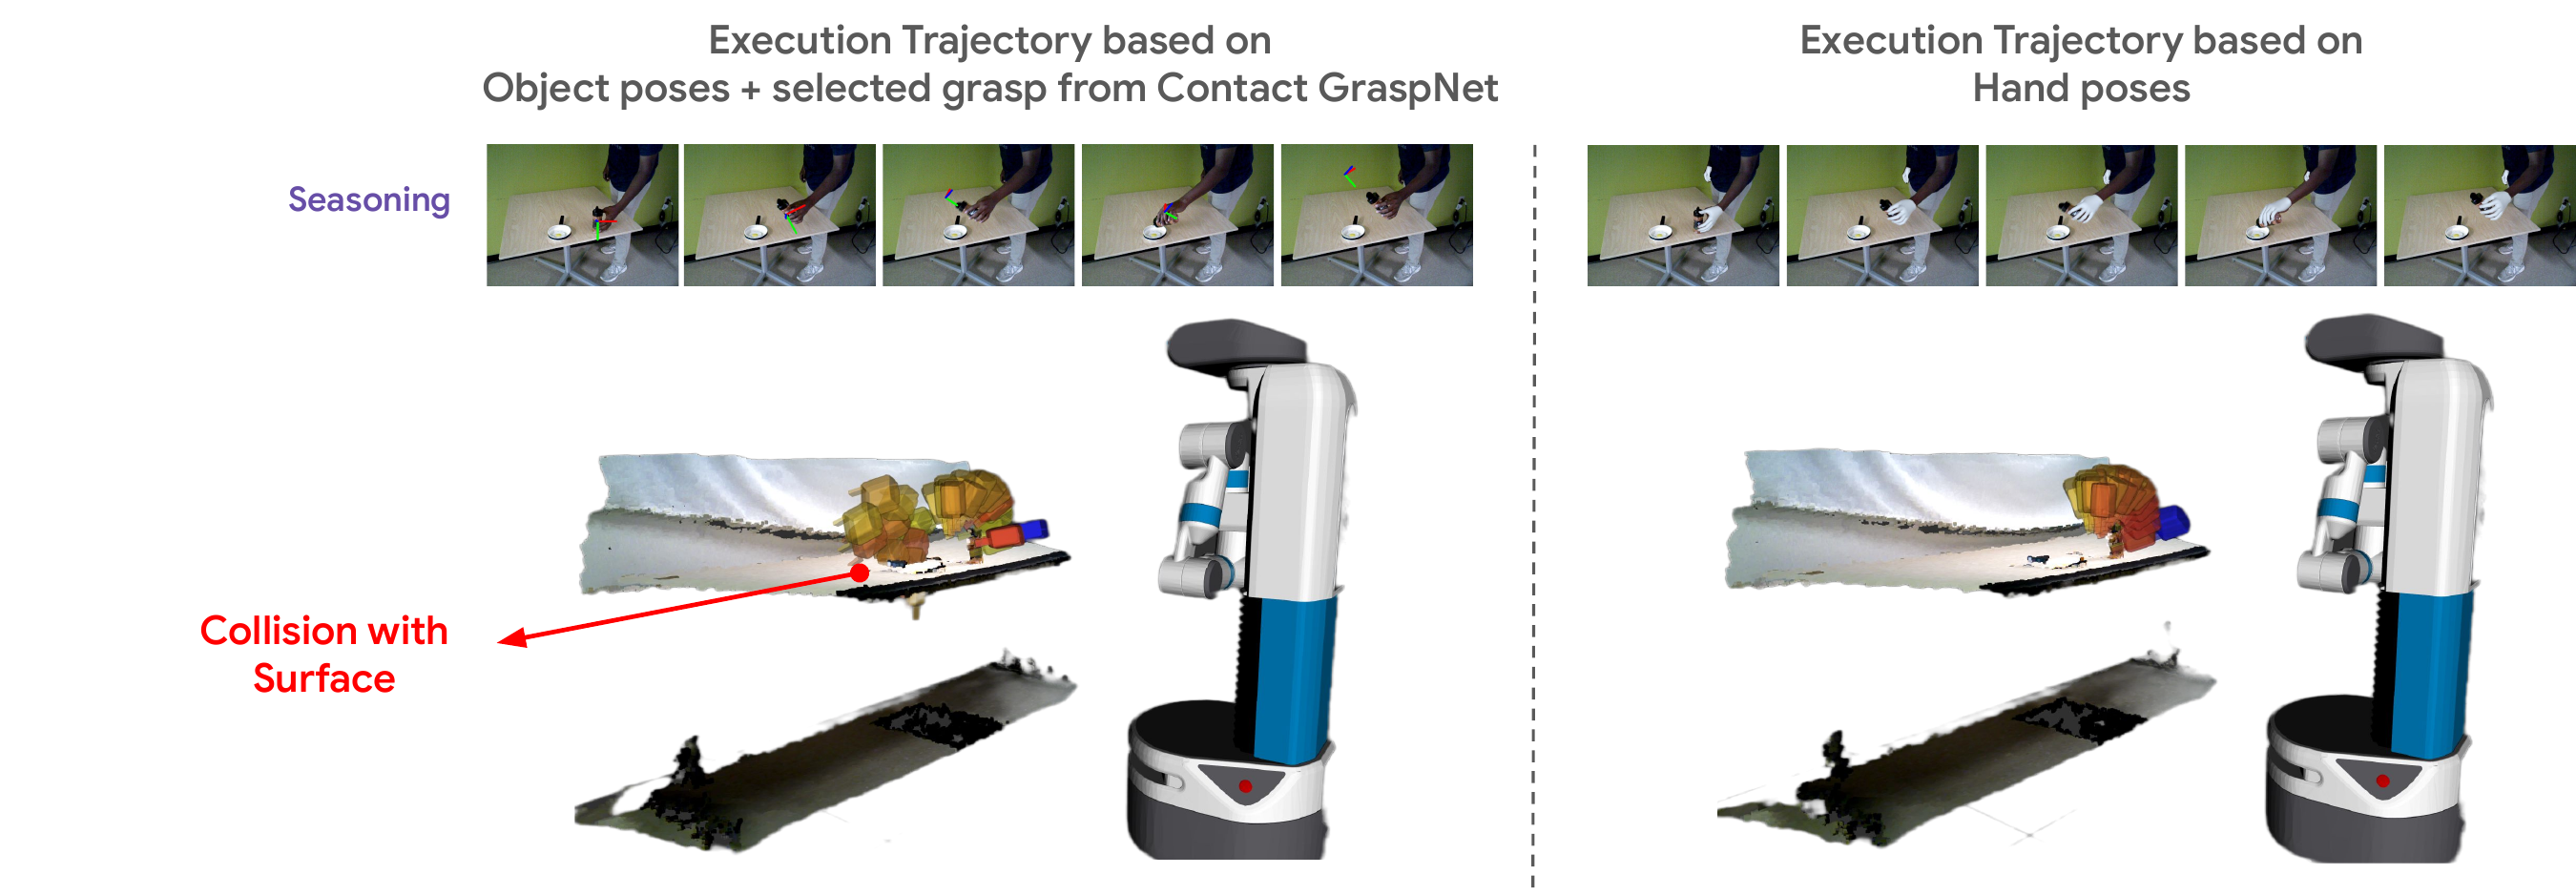}
    \caption{(left) Baseline execution: Infeasible execution trajectory waypoints colliding with the table surface. (right) Feasible execution trajectory produced using HRT1. }
    \label{fig:objtraj-collision}
\end{figure*}

\begin{figure*}[ht]
    \centering
    \includegraphics[width=\linewidth,trim={3cm 0cm 0cm 0cm},clip]{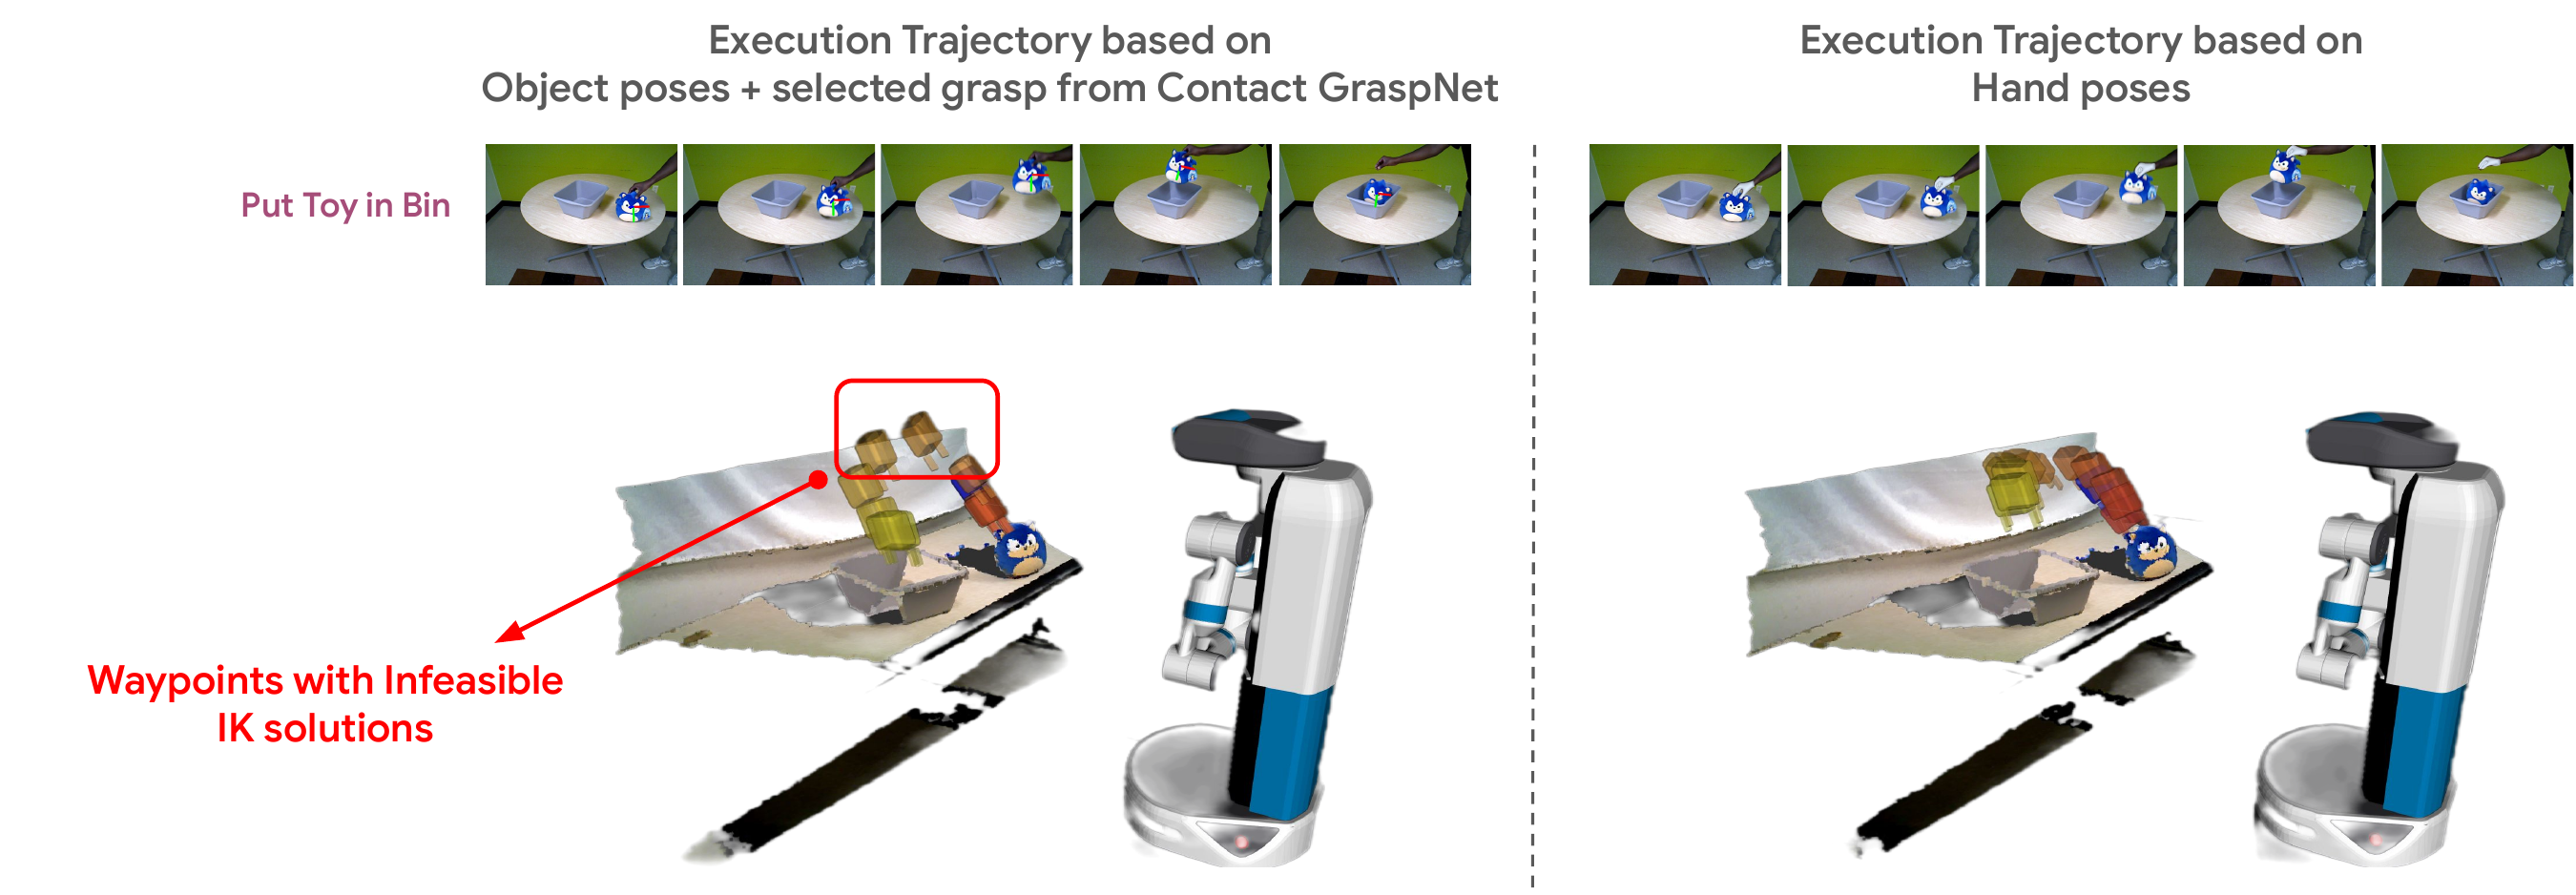}
    \caption{Caption}
    \label{fig:objtraj-noik}
\end{figure*}

\begin{figure*}
    \centering
    \includegraphics[width=\linewidth,trim={0cm 0cm 0.5cm 0cm},clip]{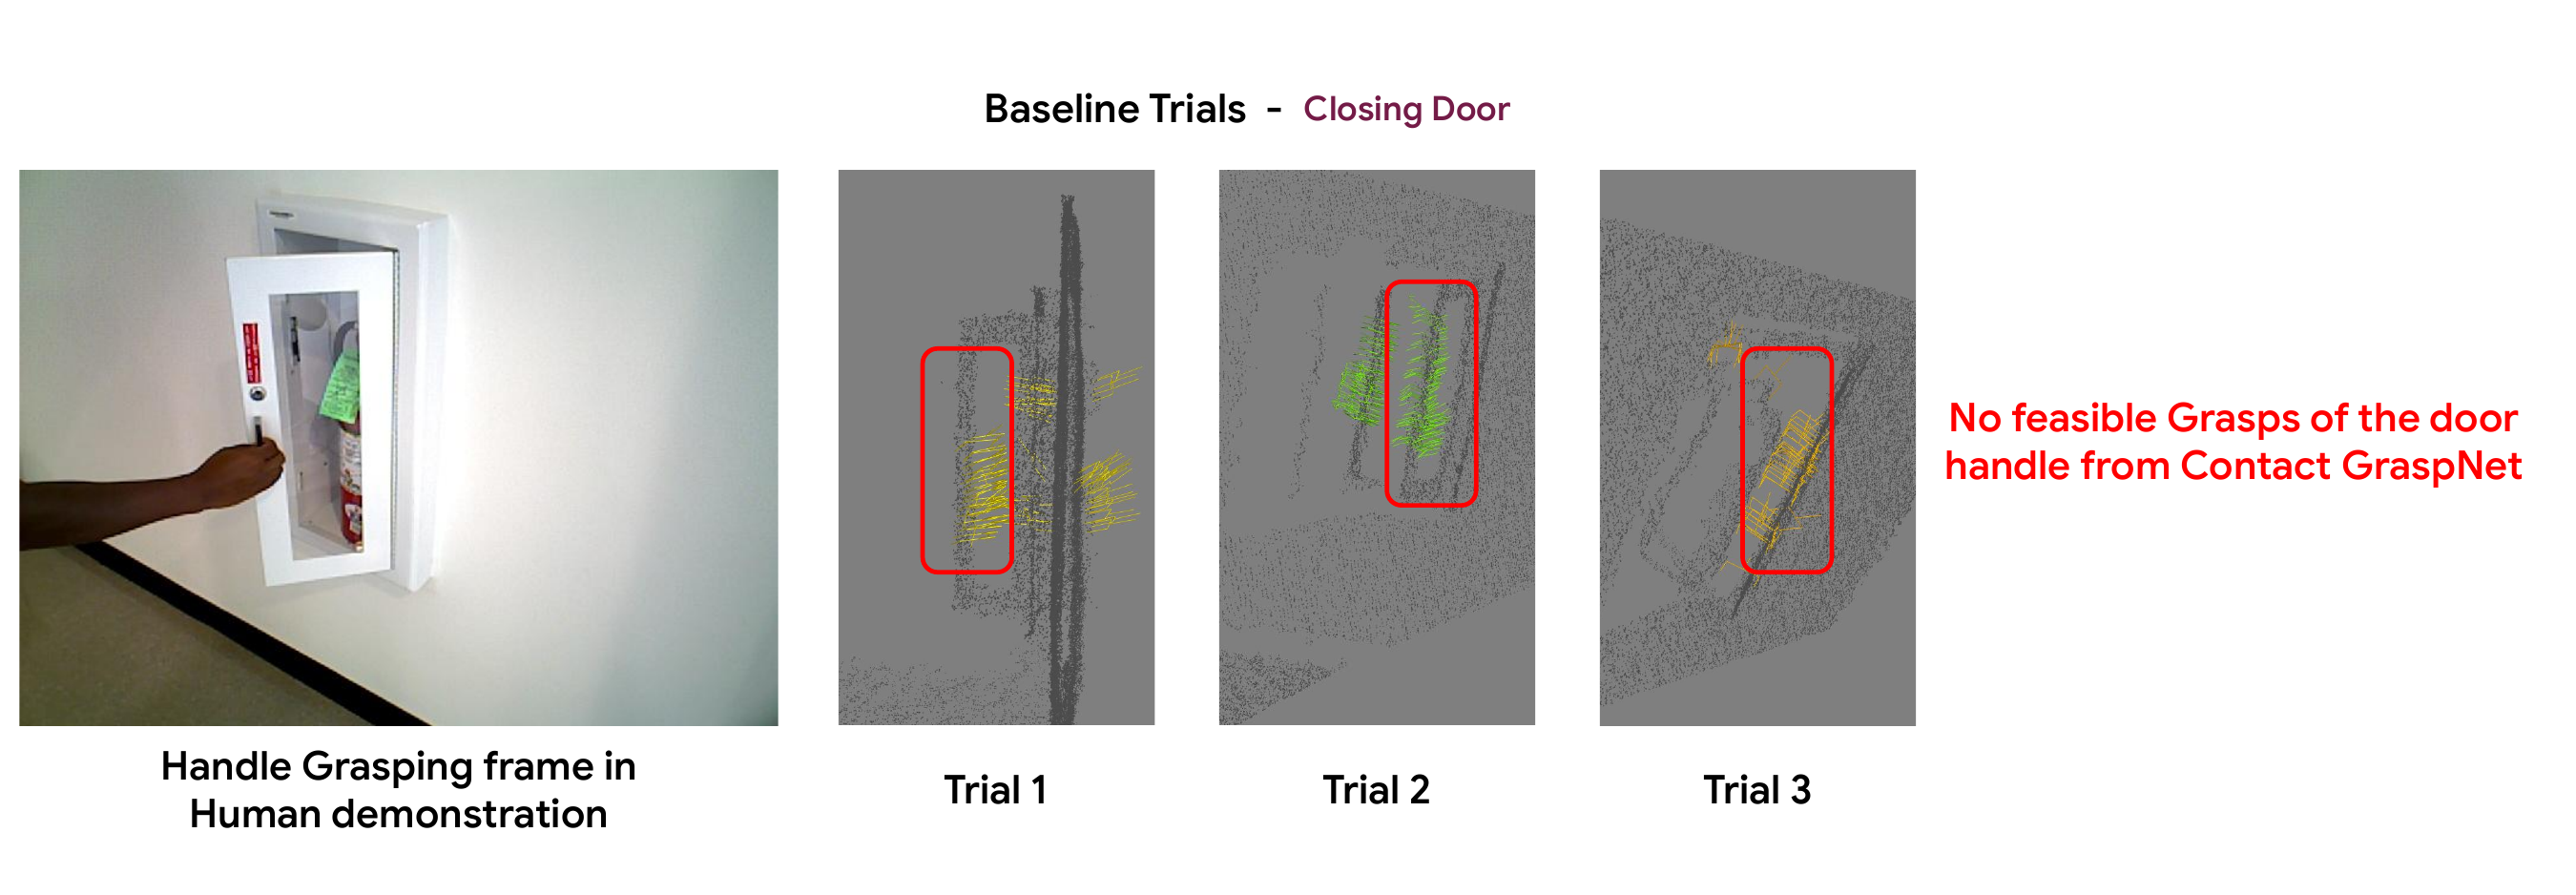}
    \caption{Illustration of grasps generated on the fire extinguisher door with a transparent glass surface. No feasible grasps are generated near the handle. }
    \label{fig:cgnet-nograsps}
\end{figure*}

\begin{figure*}
    \centering
    \includegraphics[width=\linewidth,trim={0cm 0cm 0cm 5cm},clip]{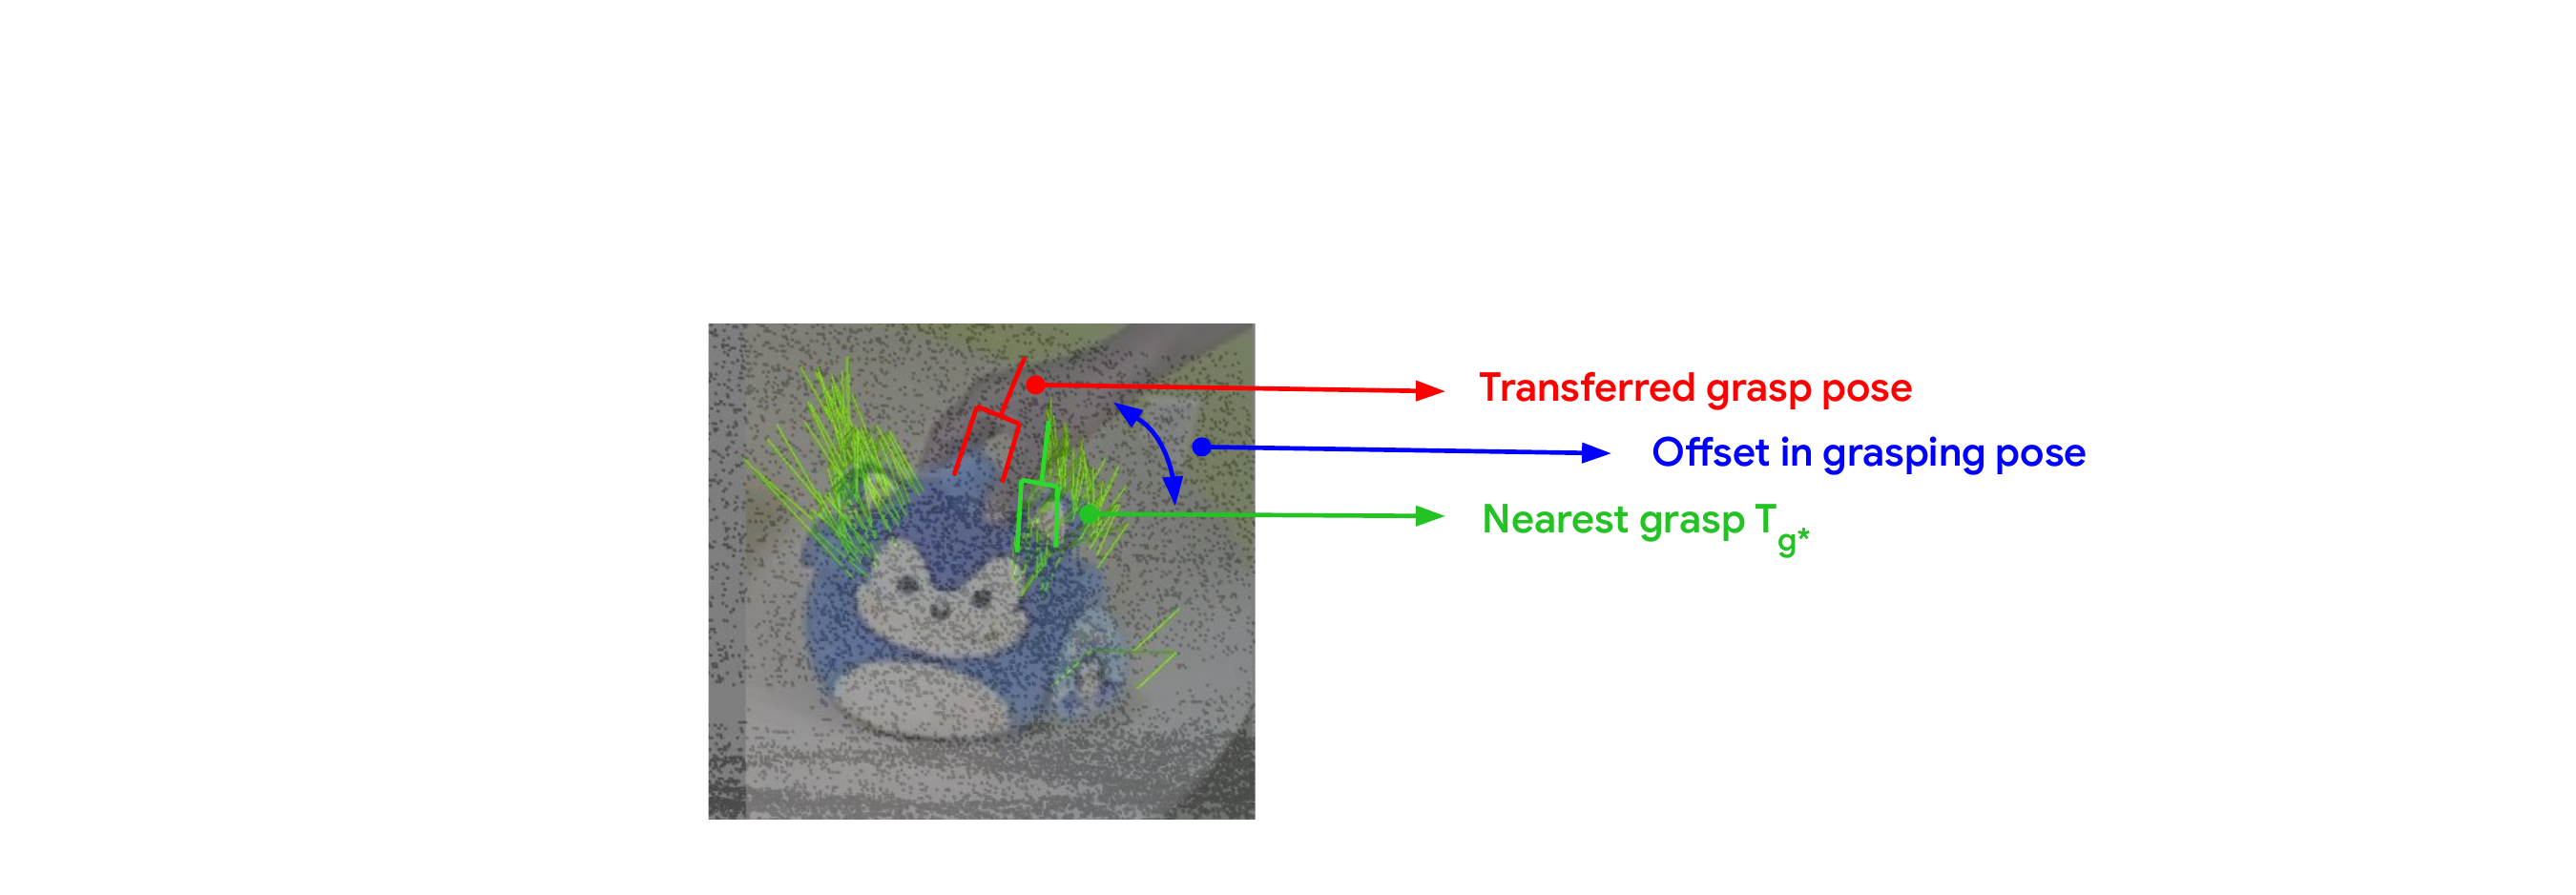}
    \caption{Offset between transferred grasp pose and the nearest }
    \label{fig:offset-grasping}    
\end{figure*}
